# Supplementary material for: Reactivity of Ambident Nucleophiles in Magnetic Fields: a Combined Conceptual DFT and Current-DFT Study
Source: arXiv:2607.22177 source file (2026-08-05)
Supplement: Supplementary file 5 [file preamble.tex]

% ========
% Preamble
% ========



% ------------------
% Scientific support
% ------------------
% Chemistry
\usepackage[version=4]{mhchem}

% Scientific typesetting
\usepackage{siunitx}
\DeclareSIUnit{\atomicunit}{a.u.}
\DeclareSIUnit{\atomicmassunit}{u}
\DeclareSIUnit{\angstrom}{\text {Å}}
\DeclareSIUnit{\cal}{cal}

% -------------
% Maths support
% -------------
\usepackage{%
  amsthm,%
  amssymb,%
  mathrsfs,%
  mathtools,%
  gensymb,%
  braket,%
  mleftright,%
  nicefrac,%
  interval%
}
\intervalconfig{%
  soft open fences%
}

\mleftright

\newcommand*\bmmax{2}
\usepackage{bm}


% --------
% Diagrams
% --------

% Colours
\usepackage[usenames, svgnames, x11names, rgb]{xcolor}

% Graphics
\usepackage{graphicx}

% --------
% Captions
% --------
\usepackage{caption, subcaption}


% ------
% Tables
% ------
\usepackage{%
  booktabs,%
  array,%
  adjustbox,%
  makecell,%
  multirow,%
  bigdelim%
}
\newcolumntype{M}[1]{>{\centering\arraybackslash}m{#1}}
\newcolumntype{L}[1]{>{\raggedright\arraybackslash}m{#1}}
\newcolumntype{R}[1]{>{\raggedleft\arraybackslash}m{#1}}

% -----
% Items
% -----
\usepackage[inline]{enumitem}


% ----------
% Hyperlinks
% ----------
\usepackage[%
  hyperfootnotes=false,%
  hypertexnames=false,%
  hidelinks,%
]{hyperref}
\hypersetup{%
  bookmarksnumbered=true,%
  colorlinks=true,%
  citecolor=teal,%
  linkcolor=Blue4,%
}


% ------------
% Bibliography
% ------------
\usepackage{mciteplus}

% ---------
% Debugging
% ---------
%\listfiles
